# Supplementary material for: Perceived Conversation Quality in Spontaneous Interactions
Source: arXiv:2207.05791 source file (2022-07-12)
Supplement: Supplementary file 1 [file PCQ_Supplementary.pdf]

# Perceived Conversation Quality in Spontaneous Interactions

## Supplementary Material

Chirag Raman\*, Navin Raj Prabhu\*, and Hayley Hung

Intelligent Systems, Delft University of Technology, Delft, Zuid-Holland, Netherlands.

\*Equal contribution.

## 1 PCQ Questionnaires

The questionnaire items below have been organized in terms of the different constituents of PCQ. The numbering before each questionnaire item indicates the ordering of the items in the original questionnaire. The original source from which the item was adapted is provided at the end of each question.

Instruction for the annotators: Use the set of questions below to annotate your perception of the individual and group’s conversation quality, as seen in the video. Each interaction aspect in the below questionnaire should be rated using a five-point likert scale (Disagree strongly (1) to Agree strongly (5)). Read the questions carefully and observe the whole group carefully before annotating the video. You are allowed to re-watch the video again if required. For the group-level measures rate the group’s behavior according to how you perceive them to behave *as a whole*. For ratings at both levels, try not to imagine how you would feel in their position, but focus on how they seem to feel based on their behaviour.

### 1.1 The Group’s Conversation Quality

#### Interpersonal Relationships

- 4 The group members seemed to have accepted and respected each other in the interaction. [1]
- 7 The group members seemed to have gotten along with each other pretty well. [1][2]
- 8 The group members were paying attention to their partners throughout the interaction. [1]
- 9 The group members attempted to get “in-sync” with their partners. [1][2]
- 10 The group members used their partner’s behavior as a guide for their own behavior. [1][2]

#### Nature of Interaction

- 1 The interaction within the group seemed smooth, natural and relaxed. [1]
- 2 The group members seemed to have enjoyed the interaction. [1]
- 3 The interaction within the group seemed forced, awkward, and strained. [1]

#### Equal Opportunity

- 5 The group members seemed to have received equal opportunity to participate freely in the interaction. [3]
- 6 The interaction involved equal participation from all group members. [3]

### 1.2 The Individual’s Experience of Conversation Quality

#### Interpersonal Relationships

- 8 The individual was paying attention to the interaction throughout. [1]
- 9 The individual seemed to have gotten along with the group pretty well. [1][2]

#### Nature of Interaction

- 1 The individual looked like they had a smooth, natural, and relaxed interaction. [1]
- 2 The individual looked like they enjoyed the interaction. [1]

- 3 The individual's interaction seemed to be forced, awkward, and strained. [1]
- 4 The individual looked like they had a pleasant and an interesting interaction. [1]
- 5 The individual appeared uncomfortable during the interaction. [1]
- 10 The individual appeared self-conscious during the interaction. [1]

### Equal Opportunity

- 6 The individual attempted to take the lead in the conversation. [2][4]
- 7 The individual looked like they experienced a free-for-all interaction. [3]

## 2 Additional Figures

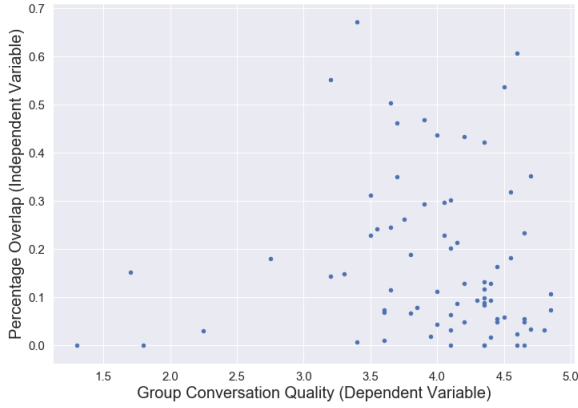

(a) Scatter plot revealing the relationship between Percentage of Overlap (Independent Variable) and the Group Conversation Quality (Dependent Variable).

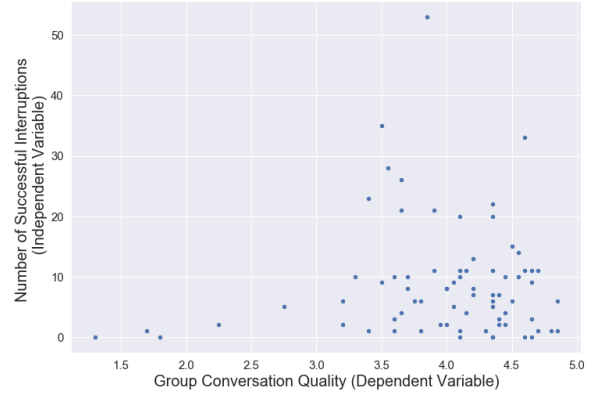

(b) Scatter plot revealing the relationship between Number of Successful Interruptions (Independent Variable) and the Group Conversation Quality (Dependent Variable).

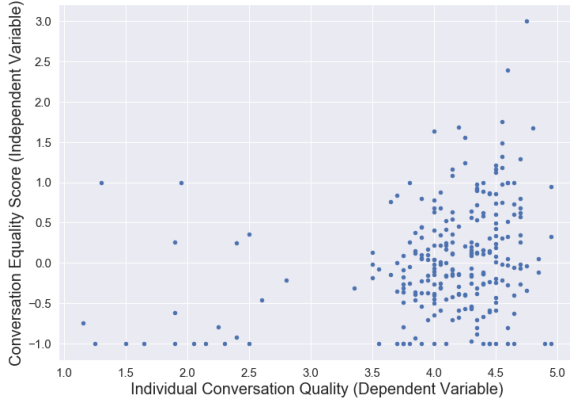

(c) Scatter plot revealing the relationship between Conversation Equality (Independent Variable) and the Individual Conversation Quality (Dependent Variable).

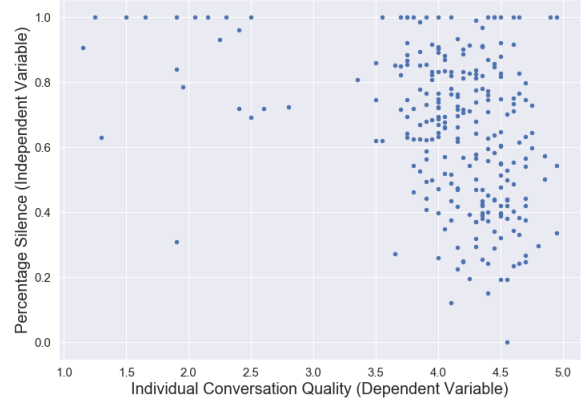

(d) Scatter plot revealing the relationship between Percentage of Silence (Independent Variable) and the Individual Conversation Quality (Dependent Variable).

**Figure S1:** Scatter plots with respect to few Independent Variables and the Dependent Variables of Conversation Quality. The scatter plots are a qualitative analysis of the independent variable's variance ( $\sigma^2$ ) conditioned to the dependent variable of Conversation Quality, and thus examine the Exogeneity and Homoscedasticity of the dataset.

## References

- [1] Ronen Cuperman and William Ickes. “Big Five Predictors of Behavior and Perceptions in Initial Dyadic Interactions: Personality Similarity Helps Extraverts and Introverts, but Hurts “Disagreeables””. In: *Journal of Personality and Social Psychology* 97.4 (2009), pp. 667–684. ISSN: 00223514. DOI: 10.1037/a0015741.
- [2] Natasha Jaques, Daniel McDuff, Yoo Lim Kim, et al. “Understanding and predicting bonding in conversations using thin slices of facial expressions and body language”. In: *Lecture Notes in Computer Science* 10011 LNAI (2016), pp. 64–74. ISSN: 16113349. DOI: 10.1007/978-3-319-47665-0\_6.
- [3] Siân E. Lindley and Andrew F. Monk. “Measuring social behaviour as an indicator of experience”. In: *Behaviour & Information Technology* 32 (Oct. 2013), pp. 968–985. ISSN: 0144-929X. DOI: 10.1080/0144929X.2011.582148.
- [4] Aleksandra Cerekovic, Oya Aran, and Daniel Gatica-Perez. “How do you like your virtual agent?: Human-agent interaction experience through nonverbal features and personality traits”. In: *Lecture Notes in Computer Science (including subseries Lecture Notes in Artificial Intelligence and Lecture Notes in Bioinformatics)* 8749 (2014), pp. 1–15. ISSN: 16113349. DOI: 10.1007/978-3-319-11839-0\_1.
